# Supplementary material for: Context-Sensitive Pointer Analysis for ArkTS
Source: arXiv:2602.00457 source file (2026-01-31)
Supplement: Supplementary file 1 [file appendix.tex]

\appendix

\section{CFG Construction}
\label{appendix:function1}
\subsection{Introduction}
\emph{scalpel.cfg} module is used to construct the control flow graphs for given python programs. The basic unit in the CFG, Block, contains a list of sequential statements that can be executed in a program without any control jumps. The `Block`s are linked by `Link` objects, which represent control flow jumps between two blocks and contain the jump conditions in the form of an expression. The two components are the fundamental data structures in the control flow graph module (\emph{scalpel.cfg}).

\subsection{How to use Control Flow Graph}
We will use the following  python program to show the CFG construction with \emph{Scalpel}. The piece of code generates the Fibonacci sequence.
\begin{lstlisting}
# example.py
def fib():
    a, b = 0, 1
    while True:
        yield a
        a, b = b, a + b

fib_gen = fib()
for _ in range(10):
    next(fib_gen)

\end{lstlisting}

To build the CFG of a source code string/source file, simply import \emph{CFGBuilder} in \emph{scalpel.cfg} and use \emph{build\_from\_src\(name, file\_path\)}. Other functions can also be used to build a CFG from a Python AST tree or a source file.

\begin{figure}
    \centering
    \begin{lstlisting}[language=python]
from scalpel.cfg import CFGBuilder

cfg = CFGBuilder().build_from_file('example.py', './example.py')

\end{lstlisting}

\end{figure}

This returns the CFG for the code in \emph{example.py} in the \emph{cfg} variable. The built CFG can be visualized with \emph{build\_visual}:

\begin{lstlisting}
cfg.build_visual('pdf')
\end{lstlisting}

Fig.~\ref{fig:cfg_example_1} is the produced \textit{exampleCFG.pdf}.
\begin{figure}[!h]
    \centering
    \includegraphics[width=0.8\linewidth]{res/fig_cfg_example_1.png}
    \caption{The control flow graph for the given source files}
    \label{fig:cfg_example_1}
\end{figure}

Apart from generating the visual graph, the CFG can be used for many other static analysis purpose.
For example, \textit{get\_calls} can be used to get all function calls in each block.

\begin{figure}
    \centering

    \begin{lstlisting}
for block in cfg:
    calls = block.get_calls()
\end{lstlisting}

\end{figure}

\subsection{Visualizations of CFG objects}

Scalpel offers some functionalities to render the CFG diagrams into PDF, PNG, JPG or SVG. Please notice this requires the graphviz package installed on your computer. Please refer to  \url{https://graphviz.readthedocs.io/en/stable/manual.html} to get it installed. 

Developers can use \textit{cfg.build\_visual()} to build a \textit{graphviz.dot.Digraph} object, then call \textit{render} function to generate the image file as shown in the following code snippet.

\begin{figure}
    \centering
    
\begin{lstlisting}[language=python]
dot = fun_cfg.build_visual('png')
dot.render("cfg_diagram", view=False)
\end{lstlisting}
\end{figure}
\subsection{Visiting Function CFGs}

In theory, there is no control flow constraint between sub-procedures such as functions. Therefore, Scalpel generates control flow graphs for every function in the given source files. Considering the nested structure of Python class and function definition, we integrate a recursive data structure for storing control flow graphs.

Take the above source code for example, scalpel will generate two CFGs. One is shown in Fig.~\ref{fig:cfg_example_1}, and the other is for the function \textit{fib}. 

We can use the following way to visit all the function CFGs in the given source. 
Please note that function CFGs can be indexed by both function name and its block id. This is due to the fact that Python allows users to define functions with same names in the same domain such as:
\begin{figure}
    \centering
    \begin{lstlisting}[language=python]
x = 0
if some condition:
   def solve():
       ...
else:
   def solve():
       ...
solve(x)
\end{lstlisting}

\end{figure}

The implementation of the function \textit{solve} can be different depending on the actual condition. Therefore, we need more than the function name to index a function CFG. Now, if we take the Fig.~\ref{fig:cfg_example_1} for example, we can visit all function CFGs in the following way and try to create a PDF file for the diagram of the CFG of function \textit{fib}: 

\begin{figure}
    \centering
    \begin{lstlisting}
    for (block_id, fun_name), fun_cfg in cfg.functioncfgs.items():
        ... # do something
        if fun_name == "fib":
            graph = fun_cfg.build_visual('png')
            graph.render("fig_cfg", view=False) 
    \end{lstlisting}

\end{figure}

\begin{figure}[!h]
    \centering
    \includegraphics[width=0.3\linewidth, height=9cm]{res/fig_cfg_example_2.png}
    \caption{The control flow graph for the function \emph{fib}}
    \label{fig:cfg_example_2}
\end{figure}

Please note, as there might be functions defined inside a function definition, you can continue perform the similar operation on the \textit{fun\_cfg} to retrieve the nested function CFGs. These CFGs can be combined for analysis. 

The tutorial code can be found at:
\url{https://github.com/SMAT-Lab/Scalpel/tree/master/examples/cfg\_tutorial.py}

\subsection{APIs}
The API documentation can be found at \url{https://smat-lab.github.io/Scalpel/scalpel/cfg.html}

\section{SSA Representations, Constant Propagation and Alias Analysis}
\label{appendix:ssa_constant}

\subsection{Introduction}
Static Single Assignment (SSA) is a technique of IR in the compiling theory\cite{rosen1988global}, it also shows great benefits to static program analysis tasks such as constant propagation, dead code elimination by providing explicit def-use chains while reducing the computational complexity .

Constant propagation is also a matured technique in static analysis. It is the process of evaluating or recognizing the actual constant values or expressions at a particular program point. This is realized by utilizing control flow and data flow information. Determining the possible values for variables before runtime greatly benefits software analysis. For instance, with conditional constant value propagation, we can detect and remove dead code or perform type checking.

In Scalpel, we implement constant propagation along with the SSA for execution efficiency.

\subsection{How to use the SSA and Constant Propagation module}

The demo input python program we will be using is as follows.
\begin{figure}
    \centering
    \begin{lstlisting}[language=python]
code_str="""
c = 10
a = -1
if c>0:
    a = a+1
else:
    a = 0
total = c+a
"""
\end{lstlisting}    
    
\end{figure}

It can be seen from the above code, the variable \textit{a} has two possible values. By utilizing the phi functions in SSA, we are able to infer that the actual return value will have two potential values. The input parameter for SSA computing is the CFG as it represents how the code blocks are organized in the program execution flow.

Please note that the function \emph{compute\_SSA} returns two dictionaries. For the first one, the key values are block numbers in the given CFG, the value is a list of dictionaries, each of which corresponds to one statement in the block. For instance, the \emph{ssa\_results[3]} (block id is 3 in this case) is a list of SSA representations for the last block. If we inspect the last block (the variable \emph{total} is assigned), the results are 

\begin{lstlisting}[language=python]
 3: [{'c': {0}, 'a': {1, 2}}]
\end{lstlisting}
This is due to that the variable \emph{a} can take values from two assignments. This can be easily observed from the following diagram. 

\begin{figure}[!h]
    \centering
      \includegraphics[width=0.6\linewidth]{res/fig_ssa_example_1.pdf}
    \caption{An example of static single assignment representations in which the variable \emph{a} in the block \#3 takes two possible values from the incoming block \#2 and \#4.}
    \label{fig:ssa_example_1}
\end{figure}

The second one named \emph{const\_dict} is the global constant values for the numbered identifiers. For instance, \emph{const\_dict[(a,0)]} is the constant value after the first assignment to variable \emph{a}. The constant values in this module are instances of Python \emph{ast.expr}. In this particular case, \emph{(a,0)} is an \emph{ast.BinOp} type and \emph{(a,1)} is an \emph{ast.Num} type.

The tutorial code can be found at: \url{https://github.com/SMAT-Lab/Scalpel/blob/master/examples/ssa\_example.py}

\subsection{Alias Analysis}

As stated above, the \emph{const\_dict} stores all the values that are assigned to given variables (renamed in this situation), therefore, alias pairs can be implemented in a simple way. The idea is to scan all the values for a particular variable and see if the value assigned to the variable is an \emph{ast.Name} object. The following code snippet shows how to find out the alias pair.

\begin{figure}
    \centering
    \begin{lstlisting}[language=python]
    ssa_results, const_dict = m_ssa.compute_SSA(cfg) 
    alias_name_pairs = []
    for name, value in const_dict.items():
        if isinstance(value, ast.Name):
        alias_name_pairs.append((name, value.id))
    \end{lstlisting}

\end{figure}
\subsection{APIs}
The API documentation can be found at \url{https://smat-lab.github.io/Scalpel/scalpel/SSA.html}

\section{Import Graph Construction}
\label{appendix:import_graph}
\subsection{Introduction}
\emph{scalpel.import\_graph} creates a data structure for describing import relationships of a python project. 
An import graph represents the dependency relationship of module files in the given project. 
This information can be important for understanding the import flow, hierarchy, encapsulation as well as software architecture.
Each node in the import graph data structure is a module file that can be manipulated to extract statements and function calls.
All the leaf nodes in the import graph can be further processed.
\subsection{How to use Import Graph}
Given three example python modules in the following example folder where three Python module files are defined. 
\begin{figure}
    \centering
        
    \begin{lstlisting}
    |-- example
           |-- module_a.py
           |-- module_b.py
           |-- module_c.py
    
    \end{lstlisting}
  
\end{figure}
  
\begin{figure}
        \centering
    \begin{lstlisting}
    #/example/module_b.py
    from .module_b import B
    from .module_c import C
    
    class A:
        def foo(self):
            return
    \end{lstlisting}

\end{figure}
\begin{figure}
    \centering
    \begin{lstlisting}
#/example/module_c.py
from .module_c import C

class B:
    def foo(self):
        return
\end{lstlisting}

\end{figure}

\begin{lstlisting}
import os

class C:
    def foo(self):
        return
\end{lstlisting}
To build the import graph of the package, import and use \emph{Tree} and \emph{ImportGraph} in \emph{scalpel.import\_graph.import\_graph}. 

\begin{figure}
    \centering
    
    \begin{lstlisting}
    from scalpel.import_graph.import_graph import Tree,ImportGraph
    
    root_node = Tree("import_graph_example_pkg")
    import_graph = ImportGraph()
    import_graph.build_dir_tree()
    module_dict = import_graph.parse_import(root_node)
    leaf_nodes = import_graph.get_leaf_nodes()
    print(len(leaf_nodes))
    
    \end{lstlisting}

\end{figure}

For each of leaf notes, we can future to extract its type information, function definition list or more meta information. The tutorial code can be found at:

\url{https://github.com/SMAT-Lab/Scalpel/blob/master/examples/import\_graph\_tutorial.py}

\subsection{APIs}
The API documentation can be found at \url{https://smat-lab.github.io/Scalpel/scalpel/import\_graph.html}

\section{Call Graph Construction}
\label{appendix:cg}
\subsection{Introduction}
A call graph depicts calling relationships between subroutines in a computer program. It is an essential component in most static analysis and can be leveraged to build more sophisticated applications such as profiling, venerability propagation and refactoring.

Please note, \emph{scalpel.call\_graph.pycg} module is a wrapper of \emph{}{PyCG}\cite{salis2021pycg} at present. It aims to construct the call graphs for given Python projects. The basic node can be either a function, a class, or a module. The edges represent calling relationships between program nodes.

\subsection{How to use the call graph module}
We use \emph{example\_pkg} package as an example and below is the folder structure of it.
\begin{figure}
    \centering
    \begin{lstlisting}
    -example_pkg
        -main.py
        -sub_folder1
            -module1.py
            -module2.py
        -sub_folder2
\end{lstlisting}
    
\end{figure}

To construct the call graph of a python application, import and use \emph{CallGraphGenerator} from \emph{scalpel.call\_graph.pycg}.

\begin{figure}
    \centering
        
    \begin{lstlisting}
    from scalpel.call_graph.pycg import CallGraphGenerator
    cg_generator = CallGraphGenerator(["main.py"], "example_pkg")
    cg_generator.analyze()
    \end{lstlisting}
    
\end{figure}
\emph{CallGraphGenerator} takes two parameters, \emph{entry\_points} and \emph{package}. \emph
{package} is the root folder of the package that we are generating a call graph for. And \emph{entry\_points} is a list of entry point files of the call graph.
Now the call graph is generated, many useful functions can be utilized to analyze the package. To output all function calls, \emph{output\_edges} can be used:

\begin{lstlisting}
edges = cg_generator.output_edges()
\end{lstlisting}

And one can use \emph{output\_internal\_mods} and \emph{output\_external\_mods} to get all internal/external modules.
\begin{figure}
    \centering
    \begin{lstlisting}
    internal_mods = cg_generator.output_internal_mods
    external_mods = cg_generator.output_external_mods
    \end{lstlisting}
    
\end{figure}

To directly operates on the call graph, one can call \emph{output}.
\begin{lstlisting}
cg = cg_generator.output()
\end{lstlisting}

\emph{scalpel.call\_graph.pycg} also provides a tool \emph{formats.Simple} to store the call graph results in the JSON format. For more functions, please refer to \url{https://pypi.org/project/pycg/}.

\begin{figure}
    \centering
    \begin{lstlisting}[language=Python]
from scalpel.call_graph.pycg import formats
import json 
formatter = formats.Simple(cg)
with open("example_results.json", "w+") as f:
    f.write(json.dumps(formatter.generate()))
\end{lstlisting}
\end{figure}

The tutorial code can be found at: \url{https://github.com/SMAT-Lab/Scalpel/blob/master/examples/cg\_tutorial.py}

\subsection{APIs}
The API documentation can be found at \url{https://smat-lab.github.io/Scalpel/scalpel/call\_graph.html}

\section{Type Inference}
\label{appendix:type_inference}
\subsection{Introduction}
Type inference module in Scalpel can identify type information for the usage context. As a dynamically type languages, the type of a Python variable is unknown until runtime (known as duck typing), making it difficult to perform type checking. Though benefiting from the coding flexibility for rapid development, Python programs can miss the opportunity to separate data from behavior and detect bugs and errors at an early stage. 

Scalpel provides a module \emph{scalpel.typeinfer} for automatic type inference to facilitate static analysis for Python programs.
\emph{scalpel.typeinfer} takes a python file or the root folder of a whole package as input, and will output a dictionary of detailed type information for each variable, including function return values and function parameters.

\subsection{How to use Type Inference}
Here is a demo input python program we will be using. The piece of code returns current working directory and is named "type\_infer\_example.py".
\begin{figure}
    \centering
    \begin{lstlisting}
    from os import getcwd
    def my_function():
        x = "Current working directory: "
        return x + getcwd()
    \end{lstlisting}
\end{figure}

To infer the types of the variables, we will use \emph{TypeInference} class in \emph{scalpel.typeinfer}.
\begin{figure}
    \centering
\begin{lstlisting}
from scalpel.typeinfer.typeinfer import TypeInference

inferer = TypeInference(name='type_infer_example.py', entry_point='type_infer_example.py')
inferer.infer_types()
inferred = inferer.get_types()
\end{lstlisting}
\end{figure}

The first parameter of \emph{TypeInference} is the desired name for the inference analyzer, and the second one is the path to a python file or the root folder of a python package. After instantiating a \emph{TypeInference} analyzer, invoke \emph{infer\_types()} method to start the inferring process. \emph{get\_types()} will return a list containing inferred type information of all variables.
The output is as follows. 
\begin{figure}
    \centering
\begin{lstlisting}
[{'file': 'type_infer_example.py', 'line_number': 4, 'function': 'my_function', 'type': {'str'}},
 {'file': 'type_infer_example.py', 'line_number': 5, 'variable': 'x', 'function': 'my_function', 'type': 'str'}]
\end{lstlisting}
\end{figure}
As shown in the output, the type of the function return value is also inferred, which is \emph{str}.

The tutorial code can be found at: \url{https://github.com/SMAT-Lab/Scalpel/blob/master/examples/type\_infer\_tutorial.py}

\subsection{APIs}
The API documentation can be found at \url{https://smat-lab.github.io/Scalpel/scalpel/typeinfer.html}
